# Supplementary material for: Optimizing Deep Learning Inference on Embedded Systems Through Adaptive Model Selection
Source: arXiv:1911.04946 source file (2019-11-09)
Supplement: Supplementary file 1 [file appendix.tex]

%!TEX root = ../main.tex
\newpage
\section*{Appendix - Artefact Description}

%\subsection*{Abstract}
Our research artefact enables the reproduction of the figures from our experimental results (Section~\ref{sec:results}). %We achieve this
%through the use of an interactive Jupyter notebook, allowing parameters to be changed to create data on request. New
%figures are created from the newly generated data in real-time.
For convenience we have provided a pre-configured live server where the notebook is
already running:
\texttt{\artefactserver} use the password \texttt{\artefactpassword}, and follow the instructions within.

\subsection{Description}
\subsubsection{Check-list}
\begin{itemize}
	\item \textbf{Run-time environment: } Ubuntu Linux and a web browser.
    \item \textbf{Hardware:} A local evaluation would require a NVIDIA Jetson TX2 platform.
	\item \textbf{Output: } Figures from the paper, and the code to create them.
	\item \textbf{Experimental workflow: } Run (or install locally) Jupyter notebook; interact with and observe results.
	\item \textbf{Experimental Customization: } Edit code in Jupyter notebook. Change which models are included in the results.
	Choose the number of images to reproduce results for. %Reproduce paper results in real-time.
	\item \textbf{Availability: } Code and data are available at:
	\url{https://zenodo.org/record/1242583#.WvAmFXUvz80}
\end{itemize}

\subsubsection{How Delivered}
An interactive Jupyter notebook on a remote server which can be used to recreate figures from our paper in real-time.
We also provide a publicly available git repository with all the code used in this work.

\subsection{Installation} \label{sec:artefact_install}
There are two ways of running the code.

\subsubsection{Hosted Jupyter notebook}
No requirements apart from a web browser.
%Access the Jupyter notebook using the pre-configured live server available at: \texttt{\artefactserver} use the password \texttt{\artefactpassword}.
You might need to ignore a browser warning about security certificates to access the notebook. High load can lead to
inconsistent results, or a long wait for results. This may occur if multiple reviewers are simultaneously trying to generate results.

\subsubsection{Local Jupyter notebook} It is also possible to create your own copy of our Jupyter notebook. For this, you will need to install Jupyter notebook locally. See
\url{http://jupyter.org/install.html} and \url{https://jupyter.readthedocs.io/en/latest/running.html} for instructions to installing and
running Jupyter Notebook, respectively.

\subsubsection{Installing from source}
To install, follow the instructions at \url{https://zenodo.org/record/1242583#.WvAmFXUvz80} This entails
Python code using the \texttt{MySQLdb}, \texttt{numpy},  \texttt{Pyro4}, \texttt{scikit-learn}, and \texttt{TensorFlow} libraries. Note
that your results will be different to ours unless you have a Jetson TX2 platform.
%For this reason we reccomend you use our pre-configured approach to evaluate the artefact.

\subsection{Experiment Workflow}
\begin{enumerate}
	\item Access the Jupyter Notebook using the method described in Section~\ref{sec:artefact_install}.
	\item From the Jupyter server page, select the checkbox next to the notebook titled
	\texttt{Artefact.ipynb}, the click ``Duplicate''.

\begin{figure}[h!b]
  \centering
  \includegraphics[width=0.45\textwidth]{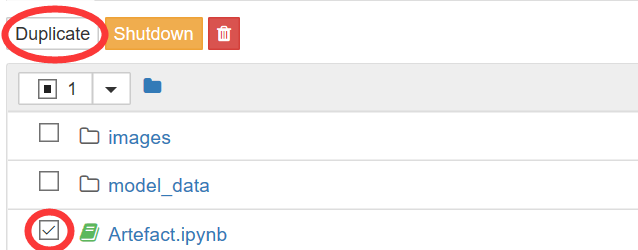}
  %\caption{}\label{}
\end{figure}

	\item Click the name of the newly created Jupyter Notebook \eg \texttt{Artefact-Copy1.ipynb}.

\begin{figure}[h!]
  \centering
  \includegraphics[width=0.45\textwidth]{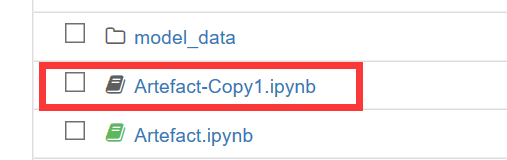}
  %\caption{}\label{}
\end{figure}

	\item Repeatedly press the \emph{play} button (tooltip is ``run cell, select below'') to step
	through each cell of the notebook.
	Alternatively, select each cell in turn and use ``Cell'' > ``Run Cell'' from the menu to run
	specific cells. Note that some cells depend on previous cells being executed. If any errors
	occur ensure all previous cells have been executed.

\begin{figure}[h!]
  \centering
  \includegraphics[width=0.45\textwidth]{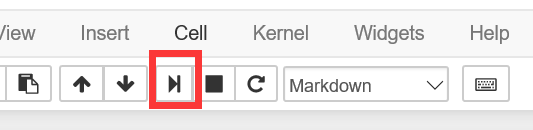}
  %\caption{}\label{}
\end{figure}
\end{enumerate}

\newpage

\subsection{Evaluation and Expected Result}
Code cells within the Jupyter Notebook display their output inline. These results can be compared
 against the values in the paper. % to check they are correct.

\subsection{Experiment Customisation}
The experiments are fully customizable, the code provided in the Jupyter Notebook
 can be edited on the spot.
Simply type your changes into the code blocks and re-run using ``Cell'' > ``Run Cells'' from the menu.
For simplicity we have provided checkboxes and sliders to change the most common variables.
Checkboxes are used to select which \DNNs or \premodel architectures  are used in each section
to produce the graphs.
Sliders are for selecting the number of images to use when validating \premodel
performance.
In the cases where less than 50k images are chosen (the total amount used in our paper), we randomly select images.
Cells will need to be re-run once any of these variables have been changed using
``Cell'' > ``Run Cells'' from the menu.
